# Supplementary material for: Comparing copy-number profiles under multi-copy amplifications and deletions
Source: arXiv:2002.11271 source file (2020-02-26)
Supplement: Supplementary file 1 [file BioMed_Central_license_agreement_doc_-_Appendix_C_.pdf]

# BioMed Central license agreement

In submitting an article to any of the journals published by BioMed Central I certify that;

1. I am authorized by my co-authors to enter into these arrangements.
2. I warrant, on behalf of myself and my co-authors, that:
   a. the article is original, has not been formally published in any other peer-reviewed journal, is not under consideration by any other journal and does not infringe any existing copyright or any other third party rights;
   b. I am/we are the sole author(s) of the article and have full authority to enter into this agreement and in granting rights to BioMed Central are not in breach of any other obligation;
   c. the article contains nothing that is unlawful, libellous, or which would, if published, constitute a breach of contract or of confidence or of commitment given to secrecy;
   d. I/we have taken due care to ensure the integrity of the article. To my/our - and currently accepted scientific - knowledge all statements contained in it purporting to be facts are true and any formula or instruction contained in the article will not, if followed accurately, cause any injury, illness or damage to the user;
3. I, and all co-authors, agree that the article, if editorially accepted for publication, shall be licensed under the Creative Commons Attribution License 4.0. In line with BioMed Central's Open Data Policy, data included in the article shall be made available under the Creative Commons 1.0 Public Domain Dedication waiver, unless otherwise stated. If the law requires that the article be published in the public domain, I/we will notify BioMed Central at the time of submission, and in such cases not only the data but also the article shall be released under the Creative Commons 1.0 Public Domain Dedication waiver. For the avoidance of doubt it is stated that sections 1 and 2 of this license agreement shall apply and prevail regardless of whether the article is published under Creative Commons Attribution License 4.0 or the Creative Commons 1.0 Public Domain Dedication waiver.

**The Creative Commons Attribution License 4.0 provides the following summary (where 'you' equals 'the user')**
**You are free to:**
**Share**—copy and redistribute the material in any medium or format
**Adapt**—remix, transform, and build upon the material for any purpose, even commercially. The licensor cannot revoke these freedoms as long as you follow the license terms.

**Under the following terms:**
**Attribution**—You must give appropriate credit, provide a link to the license, and indicate if changes were made. You may do so in any reasonable manner, but not in any way that suggests the licensor endorses you or your use.
**No additional restrictions**—You may not apply legal terms or technological measures that legally restrict others from doing anything the license permits.

**Notices:**
You do not have to comply with the license for elements of the material in the public domain or where your use is permitted by an applicable exception or limitation.
No warranties are given. The license may not give you all of the permissions necessary for your intended use. For example, other rights such as publicity, privacy, or moral rights may limit how you use the material.

**The Creative Commons 1.0 Public Domain Dedication waiver (CC0) provides the following summary:**

**No copyright**
The person who associated a work with this deed has dedicated the work to the public domain by waiving all of his or her rights to the work worldwide under copyright law, including all related and neighbouring rights, to the extent allowed by law.

You can copy, modify, distribute and perform the work, even for commercial purposes, all without asking permission. See Other information below.

**Other information**
In no way are the patent or trademark rights of any person affected by CC0, nor are the rights that other persons may have in the work or in how the work is used, such as publicity or privacy rights.
Unless expressly stated otherwise, the person who associated a work with this deed makes no warranties about the work, and disclaims liability for all uses of the work, to the fullest extent permitted by applicable law.
When using or citing the work, you should not imply endorsement by the author or the affirmer.

Comparing copy-number profiles under multi-copy amplifications and deletions (#33)
(Article title and supplement article number if known)

BMC Bioinformatics / Recomb-CG 2019
(Journal name and supplement/conference name)

MANUEL LAFOND Manuel Lafond
(Name: print and sign)

28/8/2019
(Date)
